# Supplementary material for: Multimodal Auto Validation For Self-Refinement in Web Agents
Source: arXiv:2410.00689 source file (2024-10-11)
Supplement: Supplementary file 1 [file supplemental.tex]

\subsection{Evaluator Prompts} \label{supp: eval_prompts}

\section*{Prompt 1: Validate Task (Intro)}

\begin{framed}
\texttt{
\# Task \newline
Your job is to decide whether the workflow was successfully completed, as depicted by the following sequence of screenshots. \newline

\# Workflow \newline
The workflow is: \{task\_descrip\} \newline

\# User Interface \newline
The workflow was executed within the web application shown in the screenshots. \newline

\# Workflow Demonstration \newline
You are given the following sequence of screenshots which were sourced from a demonstration of the workflow. \newline
The screenshots are presented in chronological order. \newline

Here are the screenshots of the workflow:
}
\end{framed}

\section*{Prompt 2: Validate Task (Close)}

\begin{framed}
\texttt{
\# Instructions \newline
Given what you observe in the previous sequence of screenshots, was the workflow successfully completed? \newline
If the workflow is asking a question, consider it completed successfully if you could deduce the answer to the question by viewing the screenshots. \newline
If the workflow was completed successfully, then set \{was\_completed\} to \{true/false\}. \newline

Provide your answer as a JSON dictionary with the following format: \newline
\{ \newline
    "rationale": \{rationale\}, \newline
    "was\_completed": \{true/false\} \newline
\} \newline

Please write your JSON below:
}
\end{framed}

\section*{Prompt 3: Validate VQA Task (Close)}

\begin{framed}
\texttt{
\# Instructions \newline
Given what you observed in the previous sequence of screenshots, was the workflow successfully completed? \newline
To determine this, derive a few visual questions from the task description that upon answering will help decide if the workflow was successfully completed. \newline
If the workflow is asking a question, consider it completed successfully if you can deduce the answer to the question by viewing the screenshots. \newline
If the workflow was completed successfully, then set \{was\_completed\} to \{true\}. \newline
Also, provide the visual questions and their answers as part of the response. \newline

Provide your answer as a JSON dictionary with the following format: \newline
\{ \newline
    "visual\_questions": \{list of visual questions and their answers\}, \newline
    "rationale": \{rationale\}, \newline
    "was\_completed": \{true/false\} \newline
\} \newline

Please write your JSON below:
}
\end{framed}
